# Supplementary material for: Probabilistic Regular Tree Priors for Scientific Symbolic Reasoning
Source: arXiv:2306.08506 source file (2024-06-10)
Supplement: Supplementary file 1 [file tree_languages_proofs.tex]

\section{Closure Properties of Regular Tree Languages}

We detail the proofs for the \textit{closure properties} of regular tree languages as given in literature \cite[Proposition 7.1]{rozenberg2012handbook} for the sake of completeness. These are well known results in the theoretical computer science community.

\begin{theorem}
    If $L_1, L_2 \subseteq T_\Sigma$ are regular tree languages, then $L_1 \cup L_2$ is also a regular tree language.
\end{theorem}

\begin{proof}
    This is a very clever argument.
\end{proof}

\begin{theorem}
    If $L_1, L_2 \subseteq T_\Sigma$ are regular tree languages, then $L_1 \ L_2$ is also a regular tree language.
\end{theorem}

\begin{proof}
    This is a very clever argument.
\end{proof}

\begin{theorem}
    If $L_1, L_2 \subseteq T_\Sigma$ are regular tree languages, then $L_1 \setminus L_2$ is also a regular tree language.
\end{theorem}

\begin{proof}
    This is a very clever argument.
\end{proof}

\begin{theorem}
    If $L \subseteq T_\Sigma$ is a regular tree language, then $\Bar{L} := T_\Sigma \setminus L$ is also a regular tree language.
\end{theorem}

\begin{proof}
    This is a very clever argument.
\end{proof}
